# Supplementary material for: Settling dynamics of non-Brownian suspension of spherical and cubic particles in Stokes flow
Source: arXiv:2501.08091 source file (2025-03-26)
Supplement: Supplementary file 1 [file supplementary_Material.tex]

\documentclass[a4paper,12pt,twoside]{revtex4-2}
\usepackage[utf8]{inputenc}%
\usepackage[left=0.8in,right=0.55in,top=0.4in,bottom=1.1in,includefoot,includehead]{geometry} \usepackage{amsmath}
\usepackage{graphicx}
\usepackage{xcolor} 
\usepackage{fancyhdr}
\usepackage{float}
\usepackage{siunitx}

% Includes
% \graphicspath{{Figs/}}

% Define some colors
\definecolor{brown}{rgb}{0.59, 0.29, 0.0}
\definecolor{orange}{RGB}{255,127,0}
\definecolor{brightube}{rgb}{0.82, 0.62, 0.91}

% Comments
\definecolor{darkgreen}{rgb}{0, 0.5, 0.05}

\newcommand{\deleted}[1]{}

% Set page style
 
\pagestyle{fancy}
\lhead{}
\rhead{} 
\cfoot{\thepage  \, of 2}

% Paragraph width
\usepackage{framed}

% Math commands

% Miscellaneous 

% Bold symbols

% Bold greek symbols and other

% Mathcal symbols

% Mathcal bold symbols

\begin{document}

\title{Supplemental Material: Settling dynamics of non-Brownian suspension of spherical and cubic particles in Stokes flow}

\author{Dipankar Kundu$^{1}$, Florencio Balboa Usabiaga$^{1,}$\footnote{Email address for correspondence: fbalboa@bcamath.org} and Marco Ellero$^{1,2,3}$\\
{\footnotesize $^1$Basque Center for Applied Mathematics, BCAM , Alameda de Mazarredo 14 , Bilbao 48400, Spain} \\
{\footnotesize $^2$ IKERBASQUE, Basque Foundation for Science, Calle de Maria Dias de Haro 3, 48013, Bilbao,Spain}\\
{\footnotesize $^3$ Complex Fluids Research Group, Department of Chemical Engineering, Faculty of Science and Engineering,  } \\
{\footnotesize Swansea University, Swansea SA1 8EN, United Kingdom}
}

\maketitle

\subsection*{Additional figures}

\begin{figure}[h]
  \centering
  \includegraphics[width=0.75\textwidth]{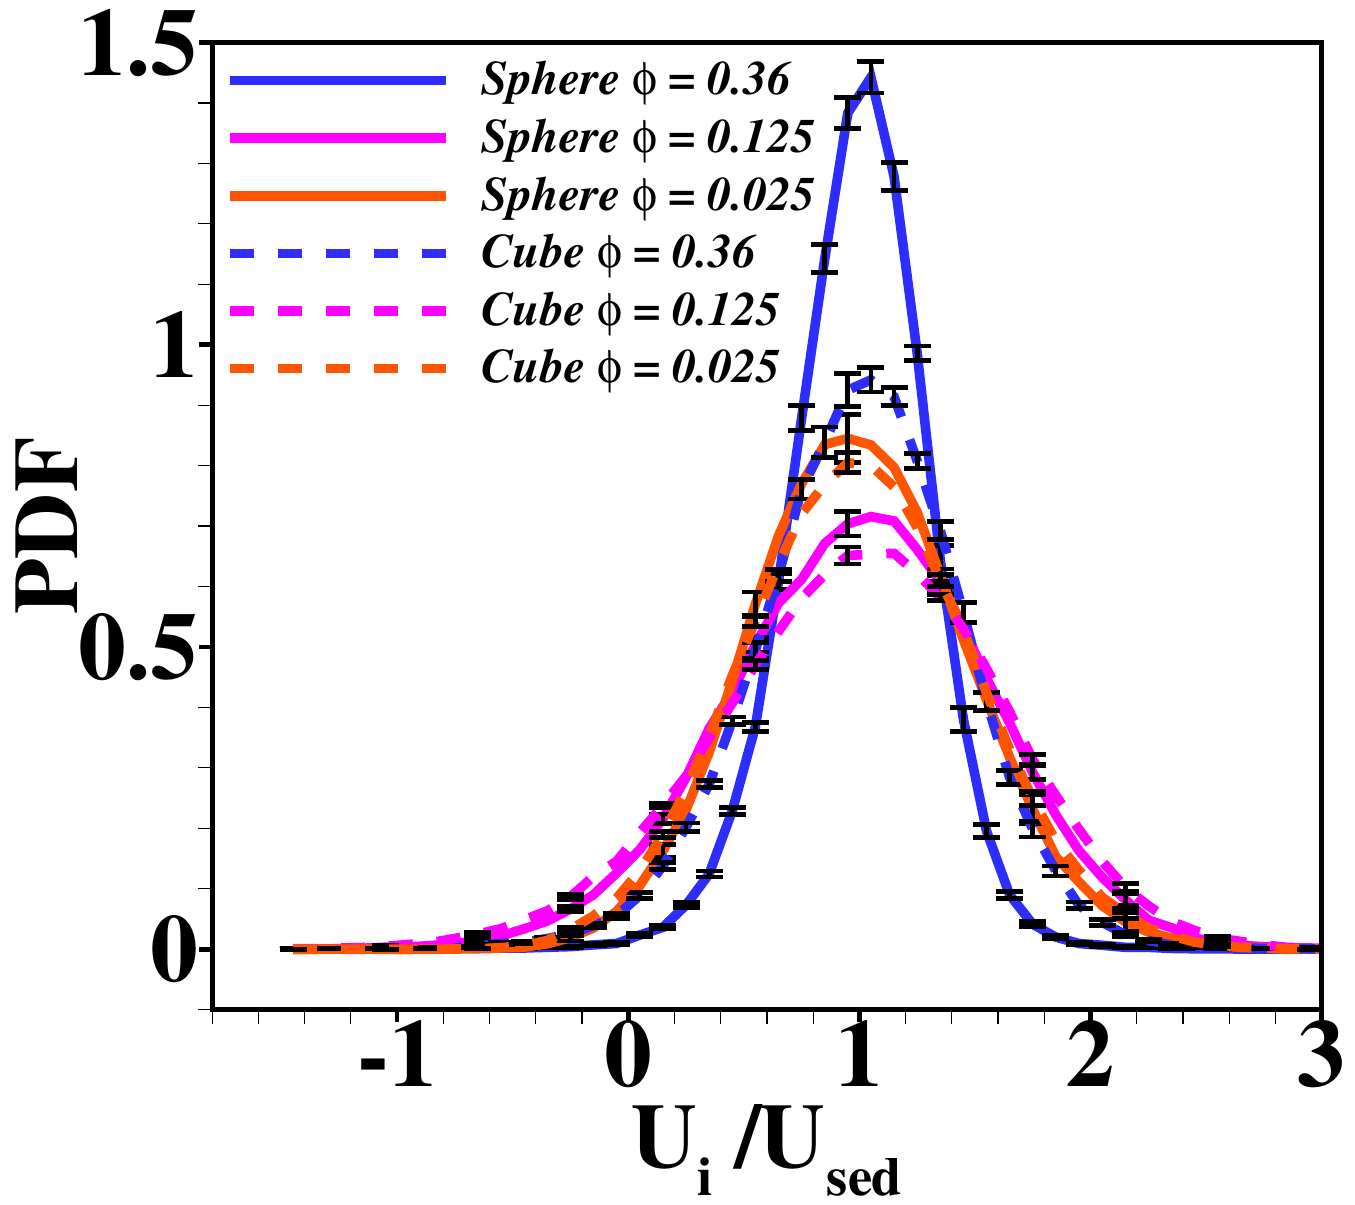}
  \caption{The probability density function (PDF) of vertical velocity is presented for both spheres and cubes for different $\phi=(0.025, 0.125, 0.36)$,
    as Fig.\ 7 in the main text.
    The PDF of spheres and cubes are similar but cubes show higher variances, or longer tails, for all volume fractions.}
\end{figure}

\begin{figure}[h]
  \centering
  \includegraphics[width=0.95\textwidth]{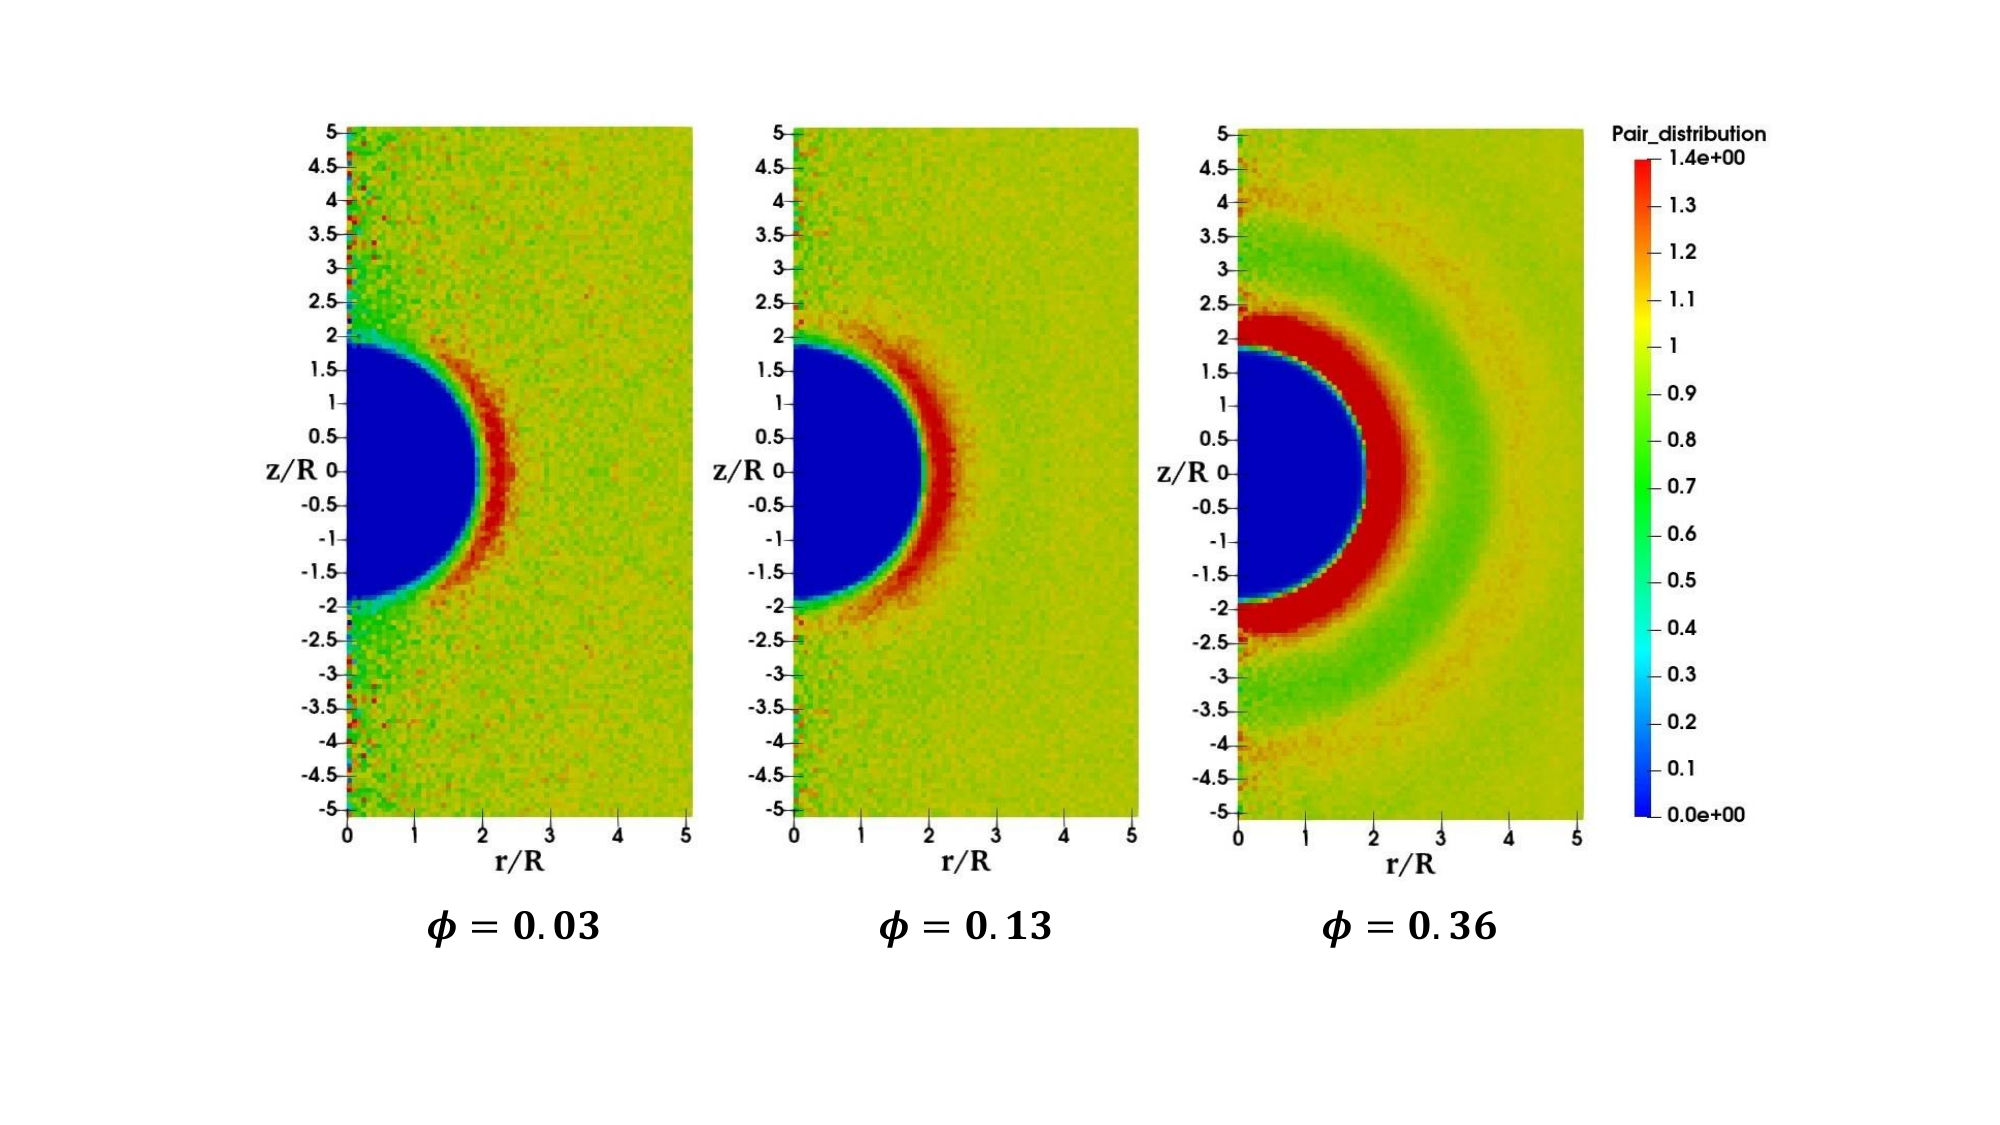}  
  \caption{Pair distribution function in cylindrical coordinates for bidisperse suspensions at various volume fraction,
    from left to right $\phi=0.03$, $\phi=0.13$, $\phi=0.36$.}
\label{pdf_mixture}  
\end{figure}

\bibliographystyle{plain}
\bibliography{biblio.bib}

\end{document}
